# Supplementary material for: AbRank: A Benchmark Dataset and Metric-Learning Framework for Antibody-Antigen Affinity Ranking
Source: arXiv:2506.17857 source file (2025-08-13)
Supplement: Supplementary file 1 [file SI.tex]

\section*{Supplementary Materials}

\subsection*{Dataset Documentation and Intended Uses}
