# Supplementary material for: AbRank: A Benchmark Dataset and Metric-Learning Framework for Antibody-Antigen Affinity Ranking
Source: arXiv:2506.17857 source file (2025-08-13)
Supplement: Supplementary file 2 [file Appendix-1.tex]

\section{Appendix-A}
\subsection{Related work}\label{sec:appendix-related-work}

% \inlinetodo{Include other antibody-antigen datasets that have been used in building machine learning models. Refer to rebuttal response to Reviewer 4.}

\textbf{Comparison of Previous Datasets} We would like to highlight our dataset, AsEP, is the largest curated AbAg benchmarking dataset to date. Existing ones either focus on general protein-protein complexes designed to develop general docking methods or are way smaller than AsEP if designed for AbAg interaction research. We summarized the sizes of existing datasets in the following table.

\begin{table}[H]
  \centering
  \caption{Comparison of Dataset Sizes Across Different Methods}
  \label{tab:dataset_sizes}
  \begin{tabular}{lc}
    \toprule
    \textbf{Method}                & \textbf{Dataset Size} \\
    \midrule
    WALLE (AsEP)                   & 1723 AbAg complexes   \\
    Wang et al. 2022~\citep{Wang2022} & 258 AbAg complexes    \\
    SAGERank~\citep{Sun2023}        & 287 AbAg complexes    \\
    CSM-AB~\citep{Myung2021}        & 472 AbAg complexes    \\
    Bepipred3.0~\citep{Bepipred}    & 582 AbAg complexes    \\
    \bottomrule
  \end{tabular}
\end{table}

In the work by \cite{Wang2022} the dataset from \cite{Zhao2018} was used, which included 257 antibody-antigen complexes, encompassing both VHVL and VHH antibodies. However, the primary focus of this research is on epitope prediction using the antigen as the input. Consequently, antibodies were not included in the predictive models, rendering the dataset unsuitable for antibody-specific epitope prediction.

For CSM-AB, as described by their supplementary information, the dataset contains 472 antibody-antigen structures including 375 Fab, 82 Nanobody and 12 scFv \citep{Myung2021}. These structures were collected from PDB, identified using Chothia annotation as in \citep{Dunbar2016}.  The authors did not describe the procedure of any further filtering steps. We assumed they included all available structures at that time with available protein-protein binding affinity information from PDBbind since the study aims to predict binding affinity.

The authors of SAGERank formed a dataset composed of 287 antibody-antigen complexes filtered by sequence identity at 95\%  \citep{Sun2023} . While the authors did not explicitly mention the antibody types, we infer from the results that these are also Fab antibodies that include both VH and VL domains. The dataset was composed mainly for docking pose ranking output by MegaDock and did not include interface clustering, i.e. epitope grouping.

SCEptRe by ~\cite{SCEptRe} is a related dataset that keeps a weekly updated collection of 3D complexes of epitope and receptor pairs, for example, antibody-antigen, TCR-pMHC, and MHC-ligand complexes derived from the Immune Epitope Database (IEDB). Our approach for clustering antibody-antigen complexes regarding their epitopes is similar to theirs, with the difference in the clustering strategy.
We cluster by antigen, then epitope group, and we allow mutated amino acids in the same epitope region because we turn the epitope sites into columns in the multiple sequence alignment. In contrast, SCEptRe clusters by antibody and then compares epitope similarity by epitope conformation using atom-pair distances via PocketMatch~\citep{PocketMatch}, which is beneficial for comparing the function of various paratopes but is less suitable for our task of predicting epitope residues.

\textbf{Sequence-based epitope predictor} We also tested purely sequence-based epitope prediction tool, for example, Bepipred3.0~\citep{Bepipred} on our dataset.
Bepipred3.0 uses ESM2 model, \texttt{esm2\_t33\_650M\_UR50D} to generate sequence embeddings and was trained on a smaller dataset of 582 antibody-antigen structures and evaluated on 15 antibody-antigen complexes.
The authors provided a relatively larger evaluation of linear B-cell epitopes derived from the Immune Epitope Database and reported an AUC-ROC of $0.693$ on the top $10\%$ of the predicted epitopes.
We tested Bepipred3.0 on our dataset and found its performance degenerates significantly, as shown in the table below.
This is not surprising because linear epitopes are consecutive positions in an antigen sequence, and this task fits better with language model design.
Additionally, as pointed out by the authors, approximately $90\%$ of epitopes (B-cell) fall into the conformational category~\citep{Bepipred}, which highlights the importance of the present benchmark dataset composed of conformational epitopes derived from filtered \AbAg~structures.
We believe these results underline the findings in our paper, showing that large language models alone, even if specialized for antibody-antigen interactions, do not encompass all the relevant information needed for epitope prediction.
% Furthermore, our model predicts epitopes and paratopes in tandem, while PLM-based approaches such as Bepipred3.0 only predict epitope residues.

\begin{table}[H]
  \centering
  \begin{tabular}{lccccc}
    \toprule
    \textbf{Confidence} Threshold & \textbf{Top 10\%} & \textbf{Top 30\%} & \textbf{Top 50\%} & \textbf{Top 70\%} & \textbf{Top 90\%} \\
    \midrule
    AUC                           & 0.693392 & 0.693392 & 0.693392 & 0.693392 & 0.693392 \\
    Balanced Accuracy             & 0.573132 & 0.636365 & 0.638755 & 0.604556 & 0.542274 \\
    MCC                           & 0.109817 & 0.140183 & 0.134689 & 0.113372 & 0.071876 \\
    Precision-Recall AUC          & 0.176429 & 0.176429 & 0.176429 & 0.176429 & 0.176429 \\
    Accuracy                      & 0.850178 & 0.701202 & 0.536947 & 0.362489 & 0.179051 \\
    Precision                     & 0.169202 & 0.141361 & 0.120547 & 0.104286 & 0.090441 \\
    Recall                        & 0.236760 & 0.553204 & 0.756607 & 0.892628 & 0.977723 \\
    F1-Score                      & 0.173370 & 0.208366 & 0.197153 & 0.179294 & 0.160151 \\
    \bottomrule
  \end{tabular}
  \caption{Bepipred3.0 results for the presented AsEP dataset. The distance cutoff was changed to 4.0Å, as this is the threshold used by Bepipred3.0. Results are shown for five confidence thresholds as described in the BepiPred-3.0 paper. Across all stringency settings and metrics, Bepipred scored lower than Walle. Furthermore, it is possible that some of the structures within the dataset are contained within the Bepipred3.0 dataset, artificially increasing scores.}
\end{table}

\subsection{Evaluation}\label{sec:appendix-evaluation}

In this work, we focus on the epitope prediction task.
We evaluate the performance of each method using consistent metrics.
Matthew's Correlation Coefficient (MCC) is highly recommended for binary classification assessments~\citep{mcc} and is especially advocated for its ability to provide equal weighting to all four values in the confusion matrix, making it a more informative metric about the classifier's performance at a given threshold than other metrics~\citep{mcc-better-1,mcc-better-2}.
We encourage the community to adopt MCC for the epitope prediction task as it takes into account true and false positives, as well as true and false negatives, offering a comprehensive measure of the performance.
It is considered superior to the AUC-ROC, which is evaluated over all thresholds.
For consistency, we also included Precision and Recall from prior studies EpiPred~\citep{epipred} and PECAN~\citep{pecan2020}, and we added Area Under the Receiver Operating Characteristic Curve (AUC-ROC) and F1 score, both are typical binary classification metrics.
For methods that predict antibody-antigen complex structures, we determine the epitopes using the same distance criterion as aforementioned.

\subsection{Steps to build antibody-antigen complex dataset}\label{sec:appendix-build-abag-dataset}

We sourced our initial dataset from AbDb (version dated September 26, 2022), containing 11,767 antibody files originally collected from the Protein Data Bank (PDB). We collected complexes numbered in Martin scheme~\citep{martin-number-scheme} and used AbM CDR definition~\citep{AbM} to identify CDR residues from the heavy and light chains of antibodies.

We extracted antibody-antigen complexes that met the following criteria: (1) both VH and VL domains are present in the antibody; (2) the antigen is a single-chain protein consisting of at least 50 amino acids; and (3) there are no unresolved CDR residues, yielding 4,081 files.

To deduplicate complexes, we used MMseqs2~\citep{mmseqs2} to cluster the complexes by heavy and light chains in antibodies and antigen sequences.
We used the \emph{easy-linclust} mode with the \emph{--cov-mode 0} option to cluster sequences;
we used the default setting for coverage of aligned cutoff at \pc{80};
we used different \emph{--min-seq-id} cutoffs for antibodies and antigens because the antibody framework regions are more conserved than the CDR regions.
We cluster heavy and light chains at \emph{--min-seq-id} cutoff of \pc{100} and \pc{70}, respectively.
We retained only one representative file for each unique set of identifiers, leading to a refined dataset of 1,725 files.

Two additional files were manually removed.
File \emph{6jmr\_1P} was removed because its CDR residues are masked with `UNK' labels and the residue identities are unknown;
file \emph{7sgm\_0P} was removed because of a non-canonical residue `DV7' in its CDR-L3 loop.

The final dataset consists of 1,723 antibody-antigen complexes.



\subsection{Pipeline to build graph dataset from AbDb}\label{sec:appendix-build-graph-dataset}

\begin{figure}[H]
  \centering
  \centerline{\includegraphics[width=.75\textwidth]{figures/appendix/build-graph-dataset-vertical.pdf}}
  \caption{Pipeline to convert an antibody-antigen complex structure into a
    graph representation.}
  \label{fig:struct-to-graph-pipeline}
  \begin{raggedright}
    % Steps
    \begin{itemize}
      \setlength\itemsep{0pt} % Set the itemsep to 0pt
      \item \textbf{Row 1}: given an AbAg complex PDB ID, retrieve `AbAg
            complex' from AbDb and `raw structure' file from PDB as input, `AbDb
            complex antigen' and `Original PDB file' in the top lane. \\
      \item \textbf{Row 2}: They are then parsed as hierarchical coordinates
            (Antigen Structure), and extract ATMSEQ and SEQRES sequences.
      \item \textbf{Row 3}: these are then passed to a set of in-house modules
            for calculating solvent access surface area (ASA), distance matrix, and
            filtering out problematic residues, which generates an
            ATMSEQ2NODES mask. The sequence alignment module aligns ATMSEQ with
            SEQRES sequences to generate a mask mapping from SEQRES to ATMSEQ.\
            The Sequence Embedding module passes SEQERS through the ESM module to
            generate embeddings. ESM requires input sequence length and therefore
            filters out sequences longer than 1021 amino acids.\\
      \item \textbf{Row 4}: holds intermediate data that we apply masks to
            generate graph data in \textbf{Row 5}.\\
      \item \textbf{Row 6}: Apply the masks to map SEQRES node embeddings
            to nodes in the graphs and calculate the edges between the graph
            nodes.\\
    \end{itemize}
  \end{raggedright}
\end{figure}

% Sequences
$U$, $V$ and $N$ denote the number of residues in the \textit{SEQRES} sequence, \textit{ATMSEQ} sequence and the graph, respectively.
\textit{thr} (at 50 residues) is the cutoff for antigen \textit{SEQRES} length. We only include antigen sequences with lengths of at least 50 residues. \textit{SEQRES} and \textit{ATMSEQ} are two different sequence representations of a protein structure.
\textit{SEQRES} is the sequence of residues in the protein chain as defined in the header section of a PDB file, and it is the complete sequence of the protein chain.
\textit{ATMSEQ} is the sequence of residues in the protein chain as defined in the ATOM section of a PDB file. In other words, it is read from the structure, and any residues in a PDB file are not resolved due to experimental issues that will be missing in the \textit{ATMSEQ} sequence. Since we are building graph representations using structures, we used \textit{ATMSEQ}. However, the input to the language models require a complete sequence, therefore we used \textit{SEQRES} to generate node embeddings, and mapped the node embeddings to the graph nodes.
We performed two pairwise sequence alignments to map such embeddings to graph vertices for a protein chain with Clustal Omega~\citep{ClustalOmega}. We first align the SEQRES sequence with the atom sequence (residues collected from the ATOM records in a PDB file) and assign residue embeddings to matched residues. Because we excluded buried residues from the graph, we aligned the sequence formed by the filtered graph vertices with the atom sequence to assign residue embeddings to vertices.
% ASA
\textit{ASA} is the solvent-accessible surface area of a residue. If a residue has an ASA value of zero, it is considered buried and will be removed from the graph.

\subsection{Dataset split}

\begin{table}[htbp]
  \centering
  \caption{Distribution of epitope to antigen surface nodes in each set.}
  \label{tab:epitope-antigen-surface-distribution}
  \begin{tabular}{llll}
    \toprule
    \textbf{Epi/Surf} & \textbf{Training} & \textbf{Validation/Test} \\
    \midrule
    0,       \pc{5}   & 320 (\pc{23} )    & 40 (\pc{24})             \\
    \pc{5} , \pc{10}  & 483 (\pc{35} )    & 60 (\pc{35})             \\
    \pc{10}, \pc{15}  & 305 (\pc{22} )    & 38 (\pc{22})             \\
    \pc{15}, \pc{20}  & 193 (\pc{14} )    & 24 (\pc{14})             \\
    \pc{20}, \pc{25}  & 53  (\pc{4}  )    & 6  (\pc{4} )             \\
    \pc{25}, \pc{30}  & 19  (\pc{1}  )    & 2  (\pc{1} )             \\
    \pc{30}, \pc{35}  & 8   (\pc{0.6})    & 0  (-      )             \\
    \pc{35}, \pc{40}  & 2   (\pc{0.1})    & 0  (-      )             \\
    sum               & 1383              & 170                      \\
    \bottomrule
  \end{tabular}
\end{table}



\subsection{Implementation details}\label{sec:appendix-implementation-details}

\textbf{Exploratory Data Analysis} We performed exploratory data analysis on the training dataset to understand the distribution of the number of residue-residue contacts in the antibody-antigen interface. We found that the number of contacts is approximately normally distributed with a mean of 43.42 and a standard deviation of 11.22 (Figure~\ref{fig:bipartite-edge-count-distribution}). We used this information to set the regularizer in the loss function to penalize the model for predicting too many or too few positive edges.

\begin{figure}[htbp]
  \centering
  \centerline{\includegraphics[width=.75\textwidth]{figures/appendix/bipartite_edge_count_distribution_fitted_normal.pdf}}
  \caption{Blue line: distribution of the number of residue-residue contacts in antibody-antigen interface across the dataset with a mean and median of 43.27 and 43.00, respectively. Red line: fitted normal distribution with mean and standard deviation of 43.27 and 10.80, respectively.}
  \label{fig:bipartite-edge-count-distribution}
\end{figure}

\textbf{Loss function} Our loss function is a weighted sum of two parts: a binary cross-entropy loss for the bipartite graph linkage reconstruction and a regularizer for the number of positive edges in the reconstructed bipartite graph.
%
\begin{align}\label{eq:loss-function}
  \text{Loss}   & = \mathcal{L}_r + \lambda \left\vert \sum^{N} \hat{e} - c \right\vert \\
  \mathcal{L}_r & = -\frac{1}{N} \sum_{i=1}^{N} \left(
  w_{\text{pos}} \cdot y_e \cdot \log(\hat{y_e}) +
  w_{\text{neg}} \cdot (1-y_e) \cdot \log(1-\hat{y_e})
  \right)
\end{align}
%
The binary cross-entropy loss $\mathcal{L}_r$ is weighted by $w_\text{pos}$ and $w_\text{neg}$ for positive and negative edges, respectively.
During hyperparameter tuning, we kept $w_\text{neg}$ fixed at $1.0$ and tuned $w_\text{pos}$.
$N$ is the total number of edges in the bipartite graph, $y_e$ denotes the true label of edge $e$, and $\hat{y}_e $ denotes the predicted probability of edge $e$.
%
The regularizer $\left\vert \sum^{N} \hat{e} - c \right\vert$ is the L1 norm of the difference between the sum of the predicted probabilities of all edges of the reconstructed bipartite graph and the mean positive edges in the training set, i.e., $c$ set to $43$. This aims to prevent an overly high false positive rate, given the fact that the number of positive edges is far less than positive edges. The regularizer weight $\lambda$ is tuned during hyperparameter tuning.

\textbf{Hyperparameters}
We carried out hyperparameter search within a predefined space that included:

\begin{itemize}[leftmargin=*]
  \item \textbf{Weights for positive edges} in bipartite graph reconstruction loss, sampled uniformly between 50 and 150.
  \item \textbf{Weights for the sum of bipartite graph positive links}, where values were drawn from a log-uniform distribution spanning $1e-7$ to $1e-4$.
  \item \textbf{Edge cutoff (x)}, defining an epitope node as any antigen node with more than x edges, with x sampled following a normal distribution with a mean of 3 and a standard deviation of 1.
  \item \textbf{Number of graph convolutional layers} in the encoder, we tested using 2 and 3 layers.
  \item \textbf{Decoder type} was varied between two configurations:
    \begin{itemize}
      \item A fully connected layer, equipped with a bias term and a dropout rate of 0.1.
      \item An inner product decoder.
    \end{itemize}
\end{itemize}

\textbf{Computing resources} All experiments were performed on a single Linux machine (Ubuntu 22.04) with one NVIDIA RTX3090 GPU card, and it took on average 3 hours for a single hyper-parameter sweeping experiment.

\subsection{Antibody-antigen complex examples}\label{sec:appendix-abag-examples}

To compare the epitopes of antibodies in AsEP, we first clustered these complexes by antigen sequences to group together antibodies targeting the same antigen via MMseqs2~\citep{mmseqs2}. Specifically, we ran MMseqs2 on antigen SEQRES sequences and using the following setup:

\begin{itemize}[leftmargin=*, topsep=0pt, itemsep=0pt, parsep=0pt]
  \item \texttt{easy-linclust} mode
  \item \texttt{cov-mode} set to \texttt{0} with the default coverage of \pc{80}: this means a sequence is considered a cluster member if it aligns at least \pc{80} of its length with the cluster representative;
  \item \texttt{min-seq-id} set to \texttt{0.7}: this means a sequence is considered a cluster member if it shares at least \pc{70} sequence identity with the cluster representative.
\end{itemize}

We encourage the reader to refer to the MMseqs2 documentation \url{https://github.com/soedinglab/mmseqs2/wiki} for more details on the parameters used.

We then identify epitopes using a distance cut-off of 4.5 Å. An antigen residue is identified as epitope if any of its heavy atoms are located within 4.5 Å of any heavy atoms from the antibody.

To compare epitopes of antibodies sharing the same antigen cluster, we aligned the antigen SEQRES sequences using Clustal Omega~\citep{ClustalOmega} (download from: \url{http://www.clustal.org/omega/}) to obtain a Multiple Sequence Alignment (MSA). Epitopes are mapped to and denoted as the MSA column indices. The epitope similarity between a pair of epitopes is then calculated as the fraction of identical columns. Two epitopes are identified as identical if they share over \texttt{0.7} of identical columns.

\begin{table}[H]
  \centering
  \caption{Antibody-Antigen Complex Examples}
  \label{tab:complex-examples}
  \begin{subtable}{\textwidth}
    \centering
    \caption{Antigen Group Information}
    \begin{tabular}{cccc}
      \toprule
      \textbf{abdbid}   & \textbf{repr}     & \textbf{size} & \textbf{epitope\_group} \\
      \midrule
      7eam\_1P & 7sn2\_0P & 183  & 0              \\
      5kvf\_0P & 5kvd\_0P & 9    & 1              \\
      5kvg\_0P & 5kvd\_0P & 9    & 2              \\
      \bottomrule
    \end{tabular}
  \end{subtable}

  \vspace{0.5cm}

  \begin{subtable}{\textwidth}
    \centering
    \caption{CDR Sequences (Heavy Chain)}
    \begin{tabular}{p{3cm} p{3.8cm} p{3.8cm} p{3.8cm}}
      \toprule
      \textbf{abdbid}  & \textbf{H1}  & \textbf{H2}  & \textbf{H3} \\
      \midrule
      7eam\_1P         & GFNIKDTYIH   & RIDPGDGDTE   & FYDYVDYGMDY \\
      5kvf\_0P         & GYTFTSSWMH   & MIHPNSGSTN   & YYYDYDGMDY  \\
      5kvg\_0P         & GYTFTSYGIS   & VIYPRSGNTY   & ENYGSVY     \\
      \bottomrule
    \end{tabular}
  \end{subtable}

  \vspace{0.5cm}

  \begin{subtable}{\textwidth}
    \centering
    \caption{CDR Sequences (Light Chain)}
    \begin{tabular}{p{3cm} p{3.8cm} p{3.8cm} p{3.8cm}}
      \toprule
      \textbf{abdbid}  & \textbf{L1}       & \textbf{L2}  & \textbf{L3}  \cr
      \midrule
      7zf4\_1P         & RASGNIHNYLA       & NAKTLAD      & QHFWSTPPWT   \\
      7zbu\_0P         & KSSQSLLYSSNQKNYLA & WASTRES      & QQYYTYPYT    \\
      7xxl\_0P         & KASQNVGTAVA       & SASNRYT      & QQFSSYPYT    \\
      \bottomrule
    \end{tabular}
  \end{subtable}

  \vspace{0.5cm}

  \begin{subtable}{\textwidth}
    \centering
    \caption{Structure Titles}
    \begin{tabular}{p{2.1cm} p{1.5cm} p{5.4cm} p{5.4cm}}
      \toprule
      \textbf{abdbid} & \textbf{resolution} & \textbf{title}                                                       & \textbf{repr\_title}                                                \\
      \midrule
      7zf4\_1P        & 1.4                 & immune complex of SARS-CoV-2 RBD and cross-neutralizing antibody 7D6 & SARS-CoV-2 Omicron variant spike protein in complex with Fab XGv265 \\
      7zbu\_0P        & 1.4                 & Zika specific antibody, ZV-64, bound to ZIKA envelope DIII           & Cryo-EM structure of zika virus complexed with Fab C10 at pH 8.0    \\
      7xxl\_0P        & 1.4                 & Zika specific antibody, ZV-67, bound to ZIKA envelope DIII           & Cryo-EM structure of zika virus complexed with Fab C10 at pH 8.0    \\
      \bottomrule
    \end{tabular}
  \end{subtable}
  \begin{raggedright}
    Here we provide three example antibody-antigen complexes from the same
    antigen group, meaning the antigen sequences from each member complex
    share sequence identity of the aligned region at least \pc{70}.
    Due to space limitation, we have broken the rows into four parts:
    Antigen group information, CDR sequences, and structure titles.\\
    \begin{itemize}
      \setlength\itemsep{0pt} % Set the itemsep to 0pt
      \item \textbf{abdbid}: AbDb ID of the group member;
      \item \textbf{repr}: AbDb ID of the antigen representative;
      \item \textbf{size}: the number of complexes in the group;
      \item \textbf{epitope\_group}: A categorical identifier of the epitope group the antibody-antigen complex belongs to;
      \item \textbf{H1}, \textbf{H2}, \textbf{H3}, \textbf{L1}, \textbf{L2}, \textbf{L3}: CDR sequences of the heavy and light chains;
      \item \textbf{resolution}: Structure resolution;
      \item \textbf{title}: Structure title of the member;
      \item \textbf{repr\_title}: Structure title of the antigen representative.
    \end{itemize}
  \end{raggedright}
\end{table}


\subsection{Multi-epitope Antigens}
We include $641$ unique antigens and $973$ epitope groups in our dataset. \cref{fig:different-ab-same-antigen} shows two examples of multi-epitope antigens in our dataset, hen egg white lysozyme (\cref{fig:different-ab-same-antigen-lysozyme}) and spike protein (\cref{fig:different-ab-same-antigen-corona}). Specifically, there are $52$ and $64$ distinct antibodies in our dataset that bind to hen egg white lysozyme and spike protein, respectively. For visual clarity, we only show five and sixteen antibodies in~\cref{fig:different-ab-same-antigen-lysozyme} and~\cref{fig:different-ab-same-antigen-corona}.

We can see that different antibodies bind to different locations on the same antigen. Details of all epitope groups are provided in the Supplementary Table \texttt{SI-AsEP-entries.csv} with annotation provided in \cref{sec:appendix-abag-examples}.

\begin{figure}[htbp]
  \centering
  \begin{subfigure}[b]{\columnwidth}
    \centering
    \includegraphics[width=200px, keepaspectratio]{figures/example-abag-complexes/hen-white-lysozyme.png}
    \caption{Five different antibodies bound to hen egg white lysozyme.
      Complexes are superimposed on the antigen structure (magenta).
      AbDb IDs of the complexes and their color: 1g7i\_0P (green), 2yss\_0P (cyan),
      1dzb\_1P (yellow), 4tsb\_0P (orange), 2iff\_0P (wheat). Antigens are colored
      in magenta.}
    \label{fig:different-ab-same-antigen-lysozyme}
  \end{subfigure}
  \vspace{\baselineskip}
  \begin{subfigure}[b]{\columnwidth}
    \centering
    \includegraphics[width=200px, keepaspectratio]{figures/example-abag-complexes/spike-protein-back.png}
    \caption{Sixteen different antibodies bound to coronavirus spike protein.
      Complexes are superimposed on the antigen structure (magenta) and
      antibodies are in different colors. AbDb IDs of the complexes:
      7k8s\_0P, 7m7w\_1P, 7d0b\_0P, 7dzy\_0P, 7ey5\_1P, 7jv4\_0P, 7k8v\_1P,
      7kn4\_1P, 7lqw\_0P, 7n8i\_0P, 7q9i\_0P, 7rq6\_0P, 7s0e\_0P, 7upl\_1P,
      7wk8\_0P, 7wpd\_0P.}
    \label{fig:different-ab-same-antigen-corona}
  \end{subfigure}
  \caption{Examples of different antibodies binding to the same antigen.}
  \label{fig:different-ab-same-antigen}
\end{figure}

\newpage

\subsection{AsEp subset for Benchmarking AlphaFold 2.3 Multimer}\label{sec:appendix-AF2-benchmark-set-files}

% \inlinetodo{Describe the method and list of AbDb files for benchmarking AF2.3M}

As documented in the AlphaFold technical notes (\url{https://github.com/google-deepmind/alphafold/blob/main/docs/technical_note_v2.3.0.md}, the AlphaFold version 2.3 Multimer (AF2M) model’s training cutoff date is September 30, 2021.
To assess AF2M's generalizability to novel epitopes not present in the training set, we identified unique epitopes by filtering based on this cutoff date.
First, we retrieved all antibody-antigen complex structures from AbDb (snapshot: 2022 September 26) and clustered the antigen sequences using MMseqs2 with the following configuration. The resulting groups are referred to as \textit{antigen clusters}:

\begin{verbatim}

    easy-cluster
    --min-seq-id=0.9  # min sequence identify
    --cov-mode=0      # coverage includes both query (cluster representative)
                      # and target (cluster member) sequence
    --coverage=0.8    # min coverage
\end{verbatim}

Next, we obtained the release date of each AbDb file, cross-referencing with the Protein Data Bank (PDB), and retained only those files in AsEP that were released after the training cutoff date.
These files were mapped to their respective \textit{antigen clusters}.

Finally, we kept only those structures where all cluster members were released after the cutoff date.
This filtering process yielded the following 76 structures:

\begin{verbatim}
AbDb files:
7pg8_1P	7lk4_3P	7rd5_1P	7tzh_1P	7zyi_0P	7pnq_0P	7rfp_1P	7lr4_0P	7tuf_1P
7pnm_0P 7rk2_1P	7seg_1P	7nx3_1P	7rk1_1P	7amq_0P	7sk9_0P	7yrf_0P	7teq_0P
7usl_0P	7vyt_1P 7tpj_0P	7ucg_2P	7lo7_0P	7l7r_1P	7vaf_0P	7t0r_0P	7ttm_0P
7lr3_1P	7tuy_0P	7a3o_0P 7wk8_0P	7ue9_0P	7stz_1P	7fbi_0P	7sfv_0P	7tdm_0P
7xw6_0P	7fbi_1P	7dce_0P	7q6c_0P 7s11_2P	7rxd_0P	7w71_1P	7sbg_0P	7zwf_0P
7r9d_0P	7oh1_0P	7po5_0P	7qu1_0P	7a3p_0P 7ttx_0P	7ura_0P	7zwm_2P	7sjn_0P
7xw7_0P	7a3t_0P	7tzh_0P	7l7r_0P	7a0w_0P	7u8m_3P 7lo8_0P	7zwm_3P	7mnl_1P
7n0a_0P	7bh8_1P	7fci_0P	8dke_0P	7daa_0P	7tug_0P	7mrz_0P 7tdn_0P	7dkj_0P
7amr_0P	7zxf_0P	7v61_1P	7teb_0P
\end{verbatim}

\subsection{AlphaFold2.3 Multimer performance}

We used the top one-ranked model generated by AlphaFold2.3 Multimer in the performance calculation in \cref{subtab:benchmark-performance-af2m}. See \cref{sec:appendix-AF2-benchmark-set-files} for the list of AbDb files used for this benchmark. The average runtime, including both constructing MSA and predicting structures, is $1.66$ hours (standard deviation: $1.19$ hours, median: $1.27$ hours).

\begin{table}[H]
    \centering
    \caption{AlphaFold2 Multimer performance on novel epitopes after its training cutoff date, 2021 September 30}
    \label{subtab:benchmark-performance-af2m}
    \begin{tabular}{p{1.5cm} p{1.9cm} p{1.9cm} p{1.9cm} p{1.9cm} p{1.9cm}}
      \toprule
      \textbf{Method}  & \textbf{MCC}  & \textbf{Precision}  & \textbf{Recall}  & \textbf{F1}   \\
      \midrule
      AF2M             & 0.262 (0.039) & 0.276 (0.033)       & 0.396 (0.043)    & 0.313 (0.036) \\
      \bottomrule
    \end{tabular}
\end{table}

\subsection{Metrics definition}\label{sec:appendix-metrics-definition}

$$
  \mathrm{MCC} = \frac{(TP \times TN - FP \times FN)}
  {\sqrt{(TP + FP) (TP + FN) (TN + FP) (TN + FN)}}
$$

$$
  \mathrm{Precision} = \frac{TP}{TP + FP}
$$

$$
  \mathrm{Recall} = \frac{TP}{TP + FN}
$$

$$
  \mathrm{F1} = \frac{2 \times \text{Precision} \times \text{Recall}}
  {\text{Precision} + \text{Recall}}
$$

TP: True Positive

FP: False Positive

TN: True Negative

FN: False Negative


\subsection{Fine-tuning ESMBind on AsEP}\label{sec:appendix-esmbind-finetuning}

The performance reported in the main text for ESMBind is derived by fine-tuning ESM2 on general protein binding sites.
We performed a further fine-tuning experiment, fine-tuning it on the presented AsEP dataset and evaluating it on the AsEP test set to enable a more direct comparison of ESMBind to WALLE.
Fine-tuning of ESMBind on AsEP was done using the Low-Rank Adaptation method~\citep{lora}.
\begin{table}[h]
  \centering
  \caption{Performance Metrics}
  \label{tab:performance_metrics}
  \begin{tabular}{c c}
    \toprule
    \textbf{Metric} & \textbf{Value}    \\
    \midrule
    MCC             & \textbf{0.103923} \\
    Accuracy        & 0.504478          \\
    AUC-ROC         & 0.584497          \\
    Precision       & 0.128934          \\
    Recall          & 0.707731          \\
    F1              & 0.213829          \\
    \bottomrule
  \end{tabular}
\end{table}
