# Supplementary material for: AbRank: A Benchmark Dataset and Metric-Learning Framework for Antibody-Antigen Affinity Ranking
Source: arXiv:2506.17857 source file (2025-08-13)
Supplement: Supplementary file 3 [file Appendix-AblationStudies.tex]

\section{Appendix: Ablation Studies}\label{sec:appendix-ablation-studies}

To investigate the impact of different components on WALLE's performance, we carried out ablation studies and described them in this section. For each model variant, we performed hyperparameter tuning and reported the evaluation performance using the model with the best performance on the validation set.

\subsection{Ablation study: replace graph component with linear layers}

To investigate whether the graph component within the WALLE framework is essential for its predictive performance, we conducted an ablation study in which the graph component was replaced with two linear layers. We refer to the model as `WALLE-L'. The first linear layer was followed by a ReLu activation function. Logits output by the second linear layer were used as input to the decoder. The rest of the model architecture remained the same.

It differs from the original WALLE model in that the input to the first linear layer is simply the concatenation of the embeddings of the antibody and antigen nodes, and the linear layers do not consider the graph structure, i.e., the spatial arrangement of either antibody or antigen residues. The model was trained using the same hyperparameters as the original WALLE model. The performance of WALLE-L was evaluated on the test set using the same metrics as the original WALLE model.

\subsection{Ablation study: WALLE with simple node encoding}

The presented WALLE model utilizes embeddings from large language models, including ESM2 \citep{ESM2} or IgFold\citep{IgFold} for representing amino acid sequences, as these models are able to capture the sequential and structural information inherent in protein sequences, providing a rich, context-aware representation of amino acids. To test the effectiveness of such embeddings in this downstream task, we conducted an ablation study where we replaced the embeddings from language models with simple node encodings. Specifically, we evaluated the performance of WALLE when using `one-hot' encoding and `BLOSUM62' encoding for amino acids in both antibody and antigen sequences.

\subsection{Ablation study: WALLE with ESM2 embeddings for both antibodies and antigens}

We also investigated whether the choice of language models can impact the predictive performance of WALLE; we conducted an ablation study to evaluate the performance of WALLE when both antibodies and antigens are represented using embeddings from the ESM2 language model~\citep{ESM2} while the original model uses AntiBERTy~\citep{IgFold} for antibodies as it is trained exclusively on antibody sequences. This also tests whether a language model trained on general protein sequences can be used for a downstream task like antibody-antigen interaction prediction.


\textbf{One-hot encoding}

One-hot encoding is a method where each residue is represented as a binary vector. Each position in the vector corresponds to a possible residue type, and the position corresponding to the residue present is marked with a 1, while all other positions are set to 0. This encoding scheme is straightforward and does not incorporate any information about the physical or chemical properties of the residues. This method tests the model's capability to leverage structural and relational information from the graph component without any assumptions introduced by more complex encoding schemes.

\textbf{BLOSUM62 encoding}

BLOSUM62 \citep{Blosum62} encoding involves using the BLOSUM62 matrix, which is a substitution matrix used for sequence alignment of proteins. In this encoding, each residue is represented by its corresponding row in the BLOSUM62 matrix. This method provides a more nuanced representation of residues, reflecting evolutionary relationships and substitution frequencies.

\subsection{Hyperparameter tuning}\label{sec:hparam-tuning}

We used the same hyperparameter search space defined in~\cref{sec:appendix-implementation-details} and performed a hyperparameter search as defined in~\cref{sec:link-prediction-baseline} for each model variant in the ablation studies.
We report the evaluation performance of the tuned model for each variant in~\cref{tab:performance-ablation}.


\begin{table*}[htbp] % Table spanning two columns
  \caption{Performance of WALLE without graph component and simple node encodings on test set from dataset split by epitope to antigen surface ratio.}
  % make the fon smaller

{\footnotesize
  \label{tab:performance-ablation}
  \centering
  \begin{tabular}{p{1.5cm} p{1.2cm} p{2.0cm} p{2.0cm} p{2.0cm} p{2.0cm} p{2.0cm}}
    \toprule
    \textbf{Method} & \textbf{Encoding} & \textbf{MCC} & \textbf{AUCROC} & \textbf{Precision} & \textbf{Recall} & \textbf{F1}    \\
    \midrule
    WALLE   & Both     & \textbf{0.264} (0.021) & \textbf{0.680} (0.014) & \textbf{0.258} (0.0117) & 0.534 (0.027)          & \textbf{0.322} (0.019) \\
    WALLE-L & Both     & 0.159 (0.016)          & 0.612 (0.011)          & 0.175 (0.011)           & 0.470 (0.024)          & 0.237 (0.014)          \\
    WALLE   & ESM2     & 0.196 (0.021)          & 0.622 (0.014)          & 0.228 (0.019)           & 0.410 (0.029)          & 0.255 (0.019)          \\
    WALLE-L & ESM2     & 0.145 (0.014)          & 0.610 (0.010)          & 0.160 (0.010)           & 0.536 (0.022)          & 0.227 (0.013)          \\
    WALLE   & One-hot  & 0.097 (0.009)          & 0.583 (0.008)          & 0.119 (0.005)           & \textbf{0.892} (0.012) & 0.203 (0.008)          \\
    WALLE   & BLOSUM   & 0.085 (0.010)          & 0.574 (0.008)          & 0.118 (0.006)           & 0.840 (0.015)          & 0.199 (0.008)          \\
    \bottomrule
  \end{tabular}
  }
  \raggedright
  The values in parentheses represent the standard error of the mean; `WALLE-L' refers to WALLE with the graph component replaced by two linear layers. `ESM2' refers to the embeddings from the ESM2 language model \texttt{esm2\_t12\_35M\_UR50D}. `One-Hot' refers to one-hot encoding of amino acids. `BLOSUM62' refers to the BLOSUM62 encoding of amino acids. `Both' refers to embedding antibodies and antigens using the \texttt{esm2\_t12\_35M\_UR50D} ESM2 model and AntiBERTy (via IgFold) language model, respectively. The best performing model is highlighted in bold.
\end{table*}

We observed that WALLE's performance with simple node encodings (`one-hot' and `BLOSUM62') is considerably lower than when using advanced embeddings from language models. This indicates that the embeddings derived from language models capture more nuanced information about the amino acids, enabling the model to better predict epitope-antigen interactions.

The degenerated performance of WALLE with simple encodings can be attributed to the lack of contextual information and structural features in these representations. The high recall but low precision values suggest that the model is unable to distinguish between true and false interactions, leading to a high number of false positives. This highlights the importance of using meaningful embeddings that capture the rich structural and sequential information present in protein sequences.

% Compare WALLE with w/o graph component -> graph component is essential

When comparing WALLE with WALLE-L (without the graph components), we observe that the model's performance drops considerably when the graph component is replaced with fully connected linear layers. This indicates that the topological information captured by the graph component also contributes to the model's predictive performance.

% Something interesting: Compare WALLE with ESM2 embeddings for both antibodies and antigens -> similar performance indicating that ESM2 embeddings are sufficient for both antibodies and antigens

We also observed that WALLE with ESM2 embeddings for both antibodies and antigens achieved similar performance to WALLE with AntiBERTy and ESM2 embeddings for antibodies and antigens, respectively. This suggests that the ESM2 embeddings somehow provide effective information for both antibodies and antigens without training exclusively on antibody sequences.
