# Supplementary material for: AbRank: A Benchmark Dataset and Metric-Learning Framework for Antibody-Antigen Affinity Ranking
Source: arXiv:2506.17857 source file (2025-08-13)
Supplement: Supplementary file 4 [file Appendix-ImpactStatement.tex]

\section{Impact Statement} \label{sec:appendix-impact-statement}
This work extends to the optimization of antibody drug development, offering a more efficient and accurate method for predicting where antibodies bind on antigens, a crucial challenge of developing therapeutic antibodies. The potential impact of this advancement is underscored by the recent approval of 136 antibody-based drugs in the United States or European Union, with 17 novel antibody therapeutics approved since January 2023 and 18 more currently under review (Antibody Society, Antibody therapeutics approved or in regulatory review in the EU or US, \url{https://www.antibodysociety.org/resources/approved-antibodies/}, 24 January 2024). These figures show the transformative impact that antibody design innovation can have on transforming the landscape of therapeutic development, offering new avenues for targeted, effective treatments that can be developed in a more time- and cost-effective manner. Such advancements hold immense potential in accelerating the creation of targeted therapies and implicitly support the broader goals of personalized medicine. Fast-tracking antibody design through \textit{in silico} epitope prediction can enable quicker responses to emerging health threats like pandemics or rapidly mutating pathogens. However, in silico predictions should not be blindly trusted and should merely guide and streamline research and diligent testing, not replace it. 

This paper presents work whose goal is to highlight antibody-specific epitope prediction as a major challenge that has not been widely studied to date, which is presented as a bipartite graph connectivity prediction task. This research stands out primarily for its development of a novel benchmarking dataset for antibody-specific epitope prediction - a resource previously unavailable in the scientific community with the potential to set a new standard in the field.

Existing methods are compared using uniform metrics and a vast room for improvement can be demonstrated across the board. A novel model is presented, which surpasses its counterparts by an order of magnitude, outperforming them by at least 5 times, validating its graph-based approach utilizing antibody and antigen structural information as well as leveraging protein language models. We provide a foundational framework that invites other researchers to further build upon and refine this baseline model, which we have demonstrated to be a highly effective approach for this task.

Open availability of the dataset and model facilitates further research and exploration in this domain, expediting the development of more advanced models. Highlighting types of antibody-antigen interactions that are disregarded in existing datasets and methods encourages the examination of shortcoming of current models. The focus on conventional antibodies in this work lays the groundwork for future exploration into epitope prediction for novel antibodies, such as nanobodies, expanding upon potential applications.
