# Supplementary material for: AbRank: A Benchmark Dataset and Metric-Learning Framework for Antibody-Antigen Affinity Ranking
Source: arXiv:2506.17857 source file (2025-08-13)
Supplement: Supplementary file 5 [file Appendix-LinkPredBaseline.tex]

\section{Appendix: Link prediction baseline}\label{sec:link-prediction-baseline}

%%%%%%%%%%%%%%%%%%%%%%%%%%%%%%%%%%%%%%%%%%%%%%%%
% Link prediction baseline performance
%%%%%%%%%%%%%%%%%%%%%%%%%%%%%%%%%%%%%%%%%%%%%%%%

While the majority of existing studies focus on node-level prediction, i.e., predicting which residues are likely to be the epitope residues, we are interested in predicting the interactions between epitope and antigen residues. We argue that, on the one hand, this would provide a more comprehensive understanding of the interaction between epitopes and antigens, and on the other hand, it would be good in terms of model interpretability. Existing methods for predicting epitope residues are mostly based on sequence information, which is not directly interpretable in terms of the interaction between epitopes and antigens.

Our hyperparameter search was conducted within a predefined space as defined in~\cref{sec:appendix-implementation-details}. We used the Bayesian optimization strategy implemented through \WB, targeting the maximization of the average bipartite graph link Matthew's Correlation Coefficient (MCC).

The optimization process was managed using the early termination functionality provided by the \WB' Hyperband method~\citep{hyperband}, with a range of minimum to maximum iterations set from 3 to 27.

The best set of hyperparameters is $2$ \textit{GCNConv} layers, a batch size of $32$, a weight for positive edges of $54.7$, a weight for the sum of positive links at approximately $5.75e-7$, and an edge cutoff of $2.38$. The resulting MCC evaluated on the test set was $0.072$ (standard error: $0.009$) for the bipartite graph link prediction task.

\begin{table*}[htbp] % Table spanning two columns
  \caption{Evaluation of WALLE on the bipartite graph link prediction task}
  \label{tab:performance-link-prediction}
  \centering
  \begin{tabular}{p{2.3cm} p{4.6cm} p{4.6cm}}
    \toprule
    Metric & Mean (Standard Error) \\
    \midrule
    MCC       & 0.072 (0.009) \\
    ROC-AUC   & 0.582 (0.011) \\
    Precision & 0.049 (0.008) \\
    Recall    & 0.167 (0.023) \\
    F1        & 0.053 (0.007) \\
    \bottomrule
  \end{tabular}
\end{table*}
