# Supplementary material for: AbRank: A Benchmark Dataset and Metric-Learning Framework for Antibody-Antigen Affinity Ranking
Source: arXiv:2506.17857 source file (2025-08-13)
Supplement: Supplementary file 6 [file Appendix-WALLEVariants.tex]

% \inlinetodo{Add the performance of WALLE with different architecture}
\begin{landscape}
\section{Appendix-B: Evaluating WALLE with Different Graph Architectures}\label{sec:appendix-eval-walle-different-graph-architecture}

\subsection{Performance of WALLE variants}

In this section, we included WALLE's performance across various graph neural network (GNN) architectures, including GAT, GCN, and GraphSAGE.
The results are organized into subsections based on two dataset split strategies: by epitope-to-antigen surface ratio and by epitope group.
In \cref{tab:diff-model-types-embeddings-epitope-prediction} and \cref{tab:diff-model-types-embeddings-bipartite-link-prediction}, the protein language models (PLM) used for generating antibody and antigen node embeddings include AntiBERTy, ESM2-35M and ESM2-650M. AntiBERTy is exclusively for generating antibody node embeddings. ESM2-35M and ESM2-650M stand for \textit{esm2\_t12\_35M\_UR50D} and \textit{esm2\_t33\_650M\_UR50D}, respectively. The performance values are shown as mean metrics with standard errors provided in parentheses.

\end{landscape}

\begin{landscape}
\begin{table*}[htbp] % Table spanning two columns
  \caption{Performance on epitope prediction}
  \label{tab:diff-model-types-embeddings-epitope-prediction}
  \begin{subtable}{\textwidth}
    \centering
    \caption{Performance on dataset split by epitope to antigen surface ratio}
    \label{subtab:diff-model-types-embeddings-epitope-prediction-epitope-ratio}
    \begin{tabular}{p{2cm} p{2.2cm} p{2cm} p{2cm} p{2cm} p{2cm} p{2cm} p{2cm}}
      \toprule
      \textbf{Method}  & \textbf{antibody PLM}          & \textbf{antigen PLM}             & \textbf{MCC}           & \textbf{Precision}     & \textbf{Recall}        & \textbf{AUCROC}        & \textbf{F1}            \\
      \midrule
      GAT         & \textcolor{ForestGreen}{AntiBERTy}  & \textcolor{Thistle}{ESM2-35M}    & 0.266 (0.023)          & 0.287 (0.020)          & 0.490 (0.027)          & 0.669 (0.014)          & 0.325 (0.020)          \\
      GCN         & \textcolor{ForestGreen}{AntiBERTy}  & \textcolor{Thistle}{ESM2-35M}    & 0.264 (0.021)          & 0.258 (0.017)          & \textbf{0.534} (0.027) & 0.680 (0.014)          & 0.322 (0.019)          \\
      GraphSAGE   & \textcolor{ForestGreen}{AntiBERTy}  & \textcolor{Thistle}{ESM2-35M}    & 0.288 (0.022)          & 0.296 (0.019)          & 0.521 (0.027)          & 0.682 (0.014)          & 0.350 (0.020)          \\
      GAT         & \textcolor{Thistle}{ESM2-35M}       & \textcolor{Thistle}{ESM2-35M}    & 0.254 (0.021)          & 0.258 (0.016)          & \textbf{0.534} (0.027) & 0.669 (0.014)          & 0.322 (0.018)          \\
      GCN         & \textcolor{Thistle}{ESM2-35M}       & \textcolor{Thistle}{ESM2-35M}    & 0.246 (0.019)          & 0.234 (0.014)          & 0.607 (0.025)          & 0.681 (0.013)          & 0.310 (0.016)          \\
      GraphSAGE   & \textcolor{Thistle}{ESM2-35M}       & \textcolor{Thistle}{ESM2-35M}    & 0.264 (0.021)          & 0.269 (0.017)          & 0.528 (0.027)          & 0.674 (0.013)          & 0.327 (0.019)          \\
      GAT         & \textcolor{ForestGreen}{AntiBERTy}  & \textcolor{NavyBlue}{ESM2-650M}  & 0.279 (0.024)          & \textbf{0.315} (0.022) & 0.437 (0.028)          & 0.664 (0.014)          & 0.333 (0.022)          \\
      GCN         & \textcolor{ForestGreen}{AntiBERTy}  & \textcolor{NavyBlue}{ESM2-650M}  & \textbf{0.305} (0.023) & 0.308 (0.019)          & 0.516 (0.028)          & \textbf{0.695} (0.015) & \textbf{0.357} (0.021) \\
      GraphSAGE   & \textcolor{ForestGreen}{AntiBERTy}  & \textcolor{NavyBlue}{ESM2-650M}  & 0.294 (0.024)          & 0.301 (0.020)          & 0.506 (0.029)          & 0.684 (0.014)          & 0.351 (0.022)          \\
      GAT         & \textcolor{NavyBlue}{ESM2-650M}     & \textcolor{NavyBlue}{ESM2-650M}  & 0.243 (0.021)          & 0.291 (0.021)          & 0.434 (0.028)          & 0.648 (0.014)          & 0.297 (0.018)          \\
      GCN         & \textcolor{NavyBlue}{ESM2-650M}     & \textcolor{NavyBlue}{ESM2-650M}  & 0.264 (0.022)          & 0.276 (0.019)          & 0.509 (0.028)          & 0.672 (0.014)          & 0.326 (0.019)          \\
      GraphSAGE   & \textcolor{NavyBlue}{ESM2-650M}     & \textcolor{NavyBlue}{ESM2-650M}  & 0.270 (0.021)          & 0.269 (0.016)          & 0.533 (0.027)          & 0.678 (0.013)          & 0.336 (0.018)          \\
      \bottomrule
    \end{tabular}
  \end{subtable}

  \vspace{1em}  % adjust space between subtables

  \begin{subtable}{\textwidth}
    \centering
    \caption{Performance on dataset split by epitope groups}
    \label{subtab:diff-model-types-embeddings-epitope-prediction-epitope-groups}
    \begin{tabular}{p{2cm} p{2.2cm} p{2cm} p{2cm} p{2cm} p{2cm} p{2cm} p{2cm}}
      \toprule
      \textbf{Method}  & \textbf{antibody PLM}          & \textbf{antigen PLM}             & \textbf{MCC}           & \textbf{Precision}     & \textbf{Recall}        & \textbf{AUCROC}        & \textbf{F1}            \\
      \midrule
      GAT         & \textcolor{ForestGreen}{AntiBERTy}  & \textcolor{Thistle}{ESM2-35M}    & 0.085 (0.017)          & 0.164 (0.016)          & 0.225 (0.021)          & 0.550 (0.010)          & 0.165 (0.015)          \\
      GCN         & \textcolor{ForestGreen}{AntiBERTy}  & \textcolor{Thistle}{ESM2-35M}    & 0.122 (0.019)          & 0.186 (0.018)          & 0.267 (0.024)          & 0.576 (0.011)          & 0.187 (0.017)          \\
      GraphSAGE   & \textcolor{ForestGreen}{AntiBERTy}  & \textcolor{Thistle}{ESM2-35M}    & 0.113 (0.016)          & 0.181 (0.015)          & 0.259 (0.020)          & 0.568 (0.010)          & 0.196 (0.015)          \\
      GAT         & \textcolor{Thistle}{ESM2-35M}       & \textcolor{Thistle}{ESM2-35M}    & 0.109 (0.016)          & 0.175 (0.016)          & 0.259 (0.023)          & 0.568 (0.010)          & 0.177 (0.015)          \\
      GCN         & \textcolor{Thistle}{ESM2-35M}       & \textcolor{Thistle}{ESM2-35M}    & 0.123 (0.017)          & 0.184 (0.016)          & \textbf{0.345} (0.025) & 0.583 (0.011)          & 0.202 (0.015)          \\
      GraphSAGE   & \textcolor{Thistle}{ESM2-35M}       & \textcolor{Thistle}{ESM2-35M}    & 0.113 (0.017)          & 0.176 (0.015)          & 0.279 (0.022)          & 0.572 (0.011)          & 0.194 (0.015)          \\
      GAT         & \textcolor{ForestGreen}{AntiBERTy}  & \textcolor{NavyBlue}{ESM2-650M}  & 0.125 (0.018)          & 0.189 (0.017)          & 0.251 (0.022)          & 0.575 (0.011)          & 0.188 (0.016)          \\
      GCN         & \textcolor{ForestGreen}{AntiBERTy}  & \textcolor{NavyBlue}{ESM2-650M}  & \textbf{0.152} (0.019) & \textbf{0.207} (0.020) & 0.299 (0.025)          & \textbf{0.596} (0.012) & \textbf{0.204} (0.018) \\
      GraphSAGE   & \textcolor{ForestGreen}{AntiBERTy}  & \textcolor{NavyBlue}{ESM2-650M}  & 0.118 (0.018)          & 0.206 (0.019)          & 0.209 (0.021)          & 0.565 (0.011)          & 0.176 (0.017)          \\
      GAT         & \textcolor{NavyBlue}{ESM2-650M}     & \textcolor{NavyBlue}{ESM2-650M}  & 0.103 (0.017)          & 0.164 (0.016)          & 0.240 (0.021)          & 0.566 (0.011)          & 0.173 (0.015)          \\
      GCN         & \textcolor{NavyBlue}{ESM2-650M}     & \textcolor{NavyBlue}{ESM2-650M}  & 0.138 (0.017)          & 0.197 (0.018)          & 0.271 (0.022)          & 0.585 (0.011)          & 0.199 (0.016)          \\
      GraphSAGE   & \textcolor{NavyBlue}{ESM2-650M}     & \textcolor{NavyBlue}{ESM2-650M}  & 0.111 (0.019)          & 0.195 (0.019)          & 0.212 (0.020)          & 0.559 (0.010)          & 0.183 (0.017)          \\
      \bottomrule
    \end{tabular}
  \end{subtable}
\end{table*}

\begin{table*}[htbp] % Table spanning two columns
  \caption{Performance on bipartite link prediction}
  \label{tab:diff-model-types-embeddings-bipartite-link-prediction}
  \begin{subtable}{\textwidth}
    \centering
    \caption{Performance on dataset split by epitope to antigen surface ratio}
    \label{subtab:diff-model-types-embeddings-bipartite-link-prediction-epitope-ratio}
    \begin{tabular}{p{2cm} p{2.2cm} p{2cm} p{2cm} p{2cm} p{2cm} p{2cm} p{2cm}}
      \toprule
      \textbf{Method}  & \textbf{antibody PLM}          & \textbf{antigen PLM}             & \textbf{MCC}           & \textbf{Precision}     & \textbf{Recall}        & \textbf{AUCROC}        & \textbf{F1}            \\
      \midrule
      GAT         & \textcolor{ForestGreen}{AntiBERTy}  & \textcolor{Thistle}{ESM2-35M}    & 0.118 (0.010)          & 0.047 (0.004)          & 0.393 (0.027)          & 0.676 (0.014)          & 0.079 (0.007)          \\
      GCN         & \textcolor{ForestGreen}{AntiBERTy}  & \textcolor{Thistle}{ESM2-35M}    & 0.114 (0.010)          & 0.049 (0.004)          & 0.343 (0.027)          & 0.657 (0.013)          & 0.080 (0.007)          \\
      GraphSAGE   & \textcolor{ForestGreen}{AntiBERTy}  & \textcolor{Thistle}{ESM2-35M}    & 0.122 (0.009)          & 0.049 (0.004)          & 0.386 (0.025)          & 0.675 (0.012)          & 0.083 (0.006)          \\
      GAT         & \textcolor{Thistle}{ESM2-35M}       & \textcolor{Thistle}{ESM2-35M}    & 0.079 (0.006)          & 0.020 (0.001)          & \textbf{0.493} (0.027) & 0.690 (0.013)          & 0.037 (0.003)          \\
      GCN         & \textcolor{Thistle}{ESM2-35M}       & \textcolor{Thistle}{ESM2-35M}    & 0.088 (0.008)          & 0.035 (0.003)          & 0.301 (0.023)          & 0.630 (0.011)          & 0.060 (0.005)          \\
      GraphSAGE   & \textcolor{Thistle}{ESM2-35M}       & \textcolor{Thistle}{ESM2-35M}    & 0.098 (0.008)          & 0.038 (0.003)          & 0.333 (0.025)          & 0.648 (0.012)          & 0.064 (0.005)          \\
      GAT         & \textcolor{ForestGreen}{AntiBERTy}  & \textcolor{NavyBlue}{ESM2-650M}  & 0.121 (0.011)          & 0.051 (0.005)          & 0.369 (0.029)          & 0.670 (0.014)          & 0.084 (0.008)          \\
      GCN         & \textcolor{ForestGreen}{AntiBERTy}  & \textcolor{NavyBlue}{ESM2-650M}  & \textbf{0.131} (0.011) & \textbf{0.062} (0.005) & 0.354 (0.029)          & 0.666 (0.014)          & \textbf{0.095} (0.008) \\
      GraphSAGE   & \textcolor{ForestGreen}{AntiBERTy}  & \textcolor{NavyBlue}{ESM2-650M}  & 0.116 (0.009)          & 0.044 (0.003)          & 0.373 (0.027)          & 0.670 (0.013)          & 0.077 (0.006)          \\
      GAT         & \textcolor{NavyBlue}{ESM2-650M}     & \textcolor{NavyBlue}{ESM2-650M}  & 0.112 (0.009)          & 0.036 (0.003)          & 0.484 (0.029)          & \textbf{0.709} (0.014) & 0.064 (0.006)          \\
      GCN         & \textcolor{NavyBlue}{ESM2-650M}     & \textcolor{NavyBlue}{ESM2-650M}  & 0.119 (0.009)          & 0.039 (0.003)          & 0.468 (0.029)          & 0.707 (0.014)          & 0.070 (0.006)          \\
      GraphSAGE   & \textcolor{NavyBlue}{ESM2-650M}     & \textcolor{NavyBlue}{ESM2-650M}  & 0.112 (0.008)          & 0.042 (0.003)          & 0.373 (0.025)          & 0.668 (0.012)          & 0.073 (0.005)          \\
      \bottomrule
    \end{tabular}
  \end{subtable}

  \vspace{1em}  % adjust space between subtables

  \begin{subtable}{\textwidth}
    \centering
    \caption{Performance on dataset split by epitope groups}
    \label{subtab:diff-model-types-embeddings-bipartite-link-prediction-epitope-groups}
    \begin{tabular}{p{2cm} p{2.2cm} p{2cm} p{2cm} p{2cm} p{2cm} p{2cm} p{2cm}}
      \toprule
      \textbf{Method}  & \textbf{antibody PLM}          & \textbf{antigen PLM}             & \textbf{MCC}           & \textbf{Precision}     & \textbf{Recall}        & \textbf{AUCROC}        & \textbf{F1}            \\
      \midrule
      GAT         & \textcolor{ForestGreen}{AntiBERTy}  & \textcolor{Thistle}{ESM2-35M}    & 0.034 (0.005)          & 0.020 (0.003)          & 0.101 (0.014)          & 0.542 (0.007)          & 0.029 (0.004)          \\
      GCN         & \textcolor{ForestGreen}{AntiBERTy}  & \textcolor{Thistle}{ESM2-35M}    & 0.048 (0.006)          & 0.020 (0.002)          & 0.195 (0.022)          & 0.581 (0.011)          & 0.034 (0.004)          \\
      GraphSAGE   & \textcolor{ForestGreen}{AntiBERTy}  & \textcolor{Thistle}{ESM2-35M}    & 0.055 (0.006)          & 0.026 (0.003)          & 0.185 (0.019)          & 0.578 (0.009)          & 0.042 (0.004)          \\
      GAT         & \textcolor{Thistle}{ESM2-35M}       & \textcolor{Thistle}{ESM2-35M}    & 0.040 (0.005)          & 0.017 (0.003)          & 0.222 (0.020)          & 0.580 (0.009)          & 0.027 (0.003)          \\
      GCN         & \textcolor{Thistle}{ESM2-35M}       & \textcolor{Thistle}{ESM2-35M}    & 0.044 (0.005)          & 0.019 (0.003)          & 0.213 (0.020)          & 0.578 (0.009)          & 0.031 (0.004)          \\
      GraphSAGE   & \textcolor{Thistle}{ESM2-35M}       & \textcolor{Thistle}{ESM2-35M}    & 0.047 (0.006)          & 0.022 (0.003)          & 0.173 (0.018)          & 0.570 (0.009)          & 0.035 (0.004)          \\
      GAT         & \textcolor{ForestGreen}{AntiBERTy}  & \textcolor{NavyBlue}{ESM2-650M}  & 0.054 (0.006)          & 0.022 (0.003)          & 0.218 (0.022)          & 0.591 (0.011)          & 0.037 (0.004)          \\
      GCN         & \textcolor{ForestGreen}{AntiBERTy}  & \textcolor{NavyBlue}{ESM2-650M}  & \textbf{0.063} (0.007) & 0.024 (0.003)          & \textbf{0.265} (0.024) & \textbf{0.613} (0.012) & 0.041 (0.004)          \\
      GraphSAGE   & \textcolor{ForestGreen}{AntiBERTy}  & \textcolor{NavyBlue}{ESM2-650M}  & 0.058 (0.007)          & \textbf{0.031} (0.003) & 0.174 (0.020)          & 0.577 (0.010)          & \textbf{0.046} (0.005) \\
      GAT         & \textcolor{NavyBlue}{ESM2-650M}     & \textcolor{NavyBlue}{ESM2-650M}  & 0.044 (0.007)          & 0.024 (0.004)          & 0.136 (0.018)          & 0.558 (0.009)          & 0.036 (0.005)          \\
      GCN         & \textcolor{NavyBlue}{ESM2-650M}     & \textcolor{NavyBlue}{ESM2-650M}  & 0.052 (0.007)          & 0.024 (0.003)          & 0.177 (0.020)          & 0.576 (0.010)          & 0.039 (0.004)          \\
      GraphSAGE   & \textcolor{NavyBlue}{ESM2-650M}     & \textcolor{NavyBlue}{ESM2-650M}  & 0.055 (0.007)          & 0.028 (0.003)          & 0.164 (0.018)          & 0.571 (0.009)          & 0.043  (0.005)         \\
      \bottomrule
    \end{tabular}
  \end{subtable}
\end{table*}
\end{landscape}



\subsection{Link prediction baseline}\label{sec:link-prediction-baseline}

%%%%%%%%%%%%%%%%%%%%%%%%%%%%%%%%%%%%%%%%%%%%%%%%
% Link prediction baseline performance
%%%%%%%%%%%%%%%%%%%%%%%%%%%%%%%%%%%%%%%%%%%%%%%%

While the majority of existing studies focus on node-level prediction, i.e., predicting which residues are likely to be the epitope residues, we are interested in predicting the interactions between epitope and antigen residues. We argue that, on the one hand, this would provide a more comprehensive understanding of the interaction between epitopes and antigens, and on the other hand, it would be good in terms of model interpretability. Existing methods for predicting epitope residues are mostly based on sequence information, which is not directly interpretable in terms of the interaction between epitopes and antigens.

Our hyperparameter search was conducted within a predefined space as defined in~\cref{sec:appendix-implementation-details}. We used the Bayesian optimization strategy implemented through \WB, targeting the maximization of the average bipartite graph link Matthew's Correlation Coefficient (MCC).

The optimization process was managed using the early termination functionality provided by the \WB' Hyperband method~\citep{hyperband}, with a range of minimum to maximum iterations set from 3 to 27.

The best performance on both tasks and dataset splits was achieved using a combination of 2 \texttt{GCNConv}-layer architecture with \texttt{AntiBERTy} and \texttt{ESM2-650M} as the antibody and antigen node embeddings, respectively.

For the epitope prediction task,
% epitope ratio dataset split
the best-performing model on the epitope-to-antigen surface ratio dataset split has model parameters that include a weight for positive edges of $140.43$, a weight for the sum of positive links of approximately $1.03 \times 10^{-5}$, and an edge cutoff of $3.39$ residues for epitope identification. The decoder applied is an inner-product operator.
% epitope group split
For the epitope group dataset split, the best-performing model uses an inner-product decoder with a weight for positive edges set to $122.64$, a weight for the sum of positive links of approximately $1.97 \times 10^{-7}$, and an edge cutoff of $9.11$ residues for epitope identification.
% result
See \cref{tab:diff-model-types-embeddings-epitope-prediction} for their performance.

For the bipartite link prediction task,
% epitope ratio data split
the best-performing model on the epitope-to-antigen surface ratio dataset split shares the same configuration as the best-performing model for the epitope prediction task on this split.
% epitope group split
On the epitope group dataset split, the best-performing model uses a weight for positive edges of $125.79$, a weight for the sum of positive links of approximately $3.99e-7$, and an edge cutoff of $18.56$ residues, also employing an inner-product decoder.
% results table
See \cref{tab:diff-model-types-embeddings-epitope-prediction} for their performance.
