# Supplementary material for: AbRank: A Benchmark Dataset and Metric-Learning Framework for Antibody-Antigen Affinity Ranking
Source: arXiv:2506.17857 source file (2025-08-13)
Supplement: Supplementary file 7 [file SI.tex]

\section*{Supplementary Materials}

\subsection*{Dataset Documentation and Intended Uses}

We provide a data card for this dataset, \texttt{DataCard-AsEP.md}, which can be downloaded using this link: \url{https://drive.google.com/file/d/1fc5kFcmUdKhyt3WmS30oLLPgnkyEeUjJ/view?usp=drive_link}

This dataset provides a unified benchmark for researchers to develop new machine-learning-based methods for the epitope prediction task.

\subsection*{Access to the Dataset}

There are two alternative sources where users can download the dataset:

\begin{itemize}
    \item The dataset can be downloaded using the Python interface provided by our GitHub Repository \href{https://github.com/biochunan/AsEP-dataset}{AsEP-dataset}. Detailed instructions on how to download the dataset are provided in the README file. Briefly, after installing the provided Python module, \texttt{asep}, the dataset can be downloaded by running the following command in the terminal:
    % \begin{lstlisting}[language=bash]
    \begin{minted}{bash}
    download-asep /path/to/directory AsEP
    # For example, to download the dataset to the current directory, run
    # download-asep . AsEP
    \end{minted}
    \item The dataset and benchmark are provided through Zenodo at \url{https://doi.org/10.5281/zenodo.11495514}.
    \item Code and Dataset interface is provided in our GitHub Repository \textbf{AsEP-dataset} at \url{https://github.com/biochunan/AsEP-dataset}.
\end{itemize}

\subsection*{Author Statement}

The authors affirm that they bear all responsibility in case of violation of rights, etc., and confirm the data license. 
The dataset is licensed under the \textbf{CC BY 4.0} License (\url{https://creativecommons.org/licenses/by/4.0/}), which is provided through the Zenodo repository. 
The code is licensed under the \textbf{MIT License} (\url{https://opensource.org/licenses/MIT}).

\subsection*{Hosting, Licensing, and Maintenance Plan}
The dataset is hosted on Zenodo, which provides a DOI (10.5281/zenodo.11495514) for the dataset. 
It also comes with a Python interface provided in our GitHub Repository, AsEP-dataset at \url{https://github.com/biochunan/AsEP-dataset}, where users can submit issues and ask questions. 
Future releases and updates will be made available through the same channels. 
As discussed in the main text, the future plan includes expanding the dataset to include novel types of antibodies, such as single-domain antibodies, and providing more sophisticated features for graph representations. 
The dataset will be maintained by the authors and will be available for a long time.

\subsection*{Links to Access the Dataset and Its Metadata}
The dataset, benchmark, and metadata are provided through \href{https://doi.org/10.5281/zenodo.11495514}{Zenodo}.

\subsection*{The Dataset}

The dataset is constructed using \texttt{pytorch-geometric Dataset} module. The dataset can be loaded using the following code:

\begin{minted}{python}
from asep.data.asepv1_dataset import AsEPv1Evaluator

evaluator = AsEPv1Evaluator()

# example
torch.manual_seed(0)
y_pred = torch.rand(1000)
y_true = torch.randint(0, 2, (1000,))

input_dict = {'y_pred': y_pred, 'y_true': y_true}
result_dict = evaluator.eval(input_dict)
print(result_dict)  # got {'auc-prc': tensor(0.5565)}
% \end{lstlisting}
\end{minted}

We also provide detailed documentation of the dataset content on Zenodo and include a description below:

\begin{itemize}
  \item \texttt{asepv1-AbDb-IDs.txt}: A text file containing the AbDb identifiers of the 1723 antibody-antigen pairs in the dataset.
  \item \texttt{asepv1\_interim\_graphs.tar.gz}: Contains 1723 \texttt{.pt} files, where each file is a dictionary with structured data:
  \begin{description}
    \item[\texttt{abdbid}] A string representing the antibody AbDb identifier.
    \item[\texttt{seqres}] A dictionary containing:
    \begin{description}
      \item[\texttt{ab}] An OrderedDict mapping string chain labels \texttt{H} and \texttt{L} to their corresponding sequence strings, representing heavy and light chains respectively.
      \item[\texttt{ag}] A dictionary mapping string chain labels to their corresponding sequence strings.
    \end{description}
    \item[\texttt{mapping}] Includes:
    \begin{description}
      \item[\texttt{ab}] Contains:
      \begin{description}
        \item[\texttt{seqres2cdr}] A binary numpy array indicating the CDR positions in the antibody sequence.
      \end{description}
      \item[\texttt{ag}] Contains:
      \begin{description}
        \item[\texttt{seqres2surf}] A binary numpy array indicating the surface residues in the antigen sequence.
        \item[\texttt{seqres2epitope}] A binary numpy array indicating the epitope residues in the antigen sequence.
      \end{description}
    \end{description}
    \item[\texttt{embedding}] Comprises:
    \begin{description}
      \item[\texttt{ab}] Includes embeddings computed using the AntiBERTy model and ESM2 model for the antibody sequences.
      \item[\texttt{ag}] Includes embeddings for the antigen sequences computed using the ESM2 model.
    \end{description}
    \item[\texttt{edges}] Describes the interactions:
    \begin{description}
      \item[\texttt{ab}] A sparse coo tensor representing the binary edges between the CDR residues.
      \item[\texttt{ag}] A sparse coo tensor representing the binary edges between the surface residues.
    \end{description}
    \item[\texttt{stats}] Metadata about each antibody-antigen pair, including counts of CDR, surface, and epitope residues, and the epitope-to-surface ratio.
  \end{description}
  \item \texttt{structures.tar.gz}: Contains \texttt{1723} pdb structures, each named using the AbDb identifier.
  \item \texttt{split\_dict.pt}: Contains the \texttt{train}/\texttt{val}/\texttt{test} splits of the dataset, with splits based on the epitope ratio and epitope group of the antigen.
\end{itemize}

\subsection*{Long-term Preservation}

The current version of the dataset and benchmark are provided through Zenodo, which provides long-term storage. 
Future versions will be made available through the same channel and users are encouraged to submit queries and issues through the issues channel on the GitHub repository.

\subsection*{Explicit License}

The dataset is licensed under the \textbf{CC BY 4.0} license (\url{https://creativecommons.org/licenses/by/4.0/}), which is provided through the Zenodo repository. 
The code is licensed under the MIT License \url{https://opensource.org/licenses/MIT}.

\subsection*{Benchmarks}

Detailed benchmark experiments and results are provided on Zenodo (\url{https://doi.org/10.5281/zenodo.11495514}), and the file \texttt{benchmark.zip} contains the instructions on how to reproduce the results. 
To run ESMFold, EpiPred, and MaSIF-Site, we provided docker images on the Zenodo repository or instructions on how to obtain them from DockerHub. 
The benchmark results are reproducible by following the instructions provided in the zip file. 
For the method WALLE and its variants used in the ablation studies, their configuration YAML files and the trained models are also provided on Zenodo.
